# Supplementary material for: Suppression of Brillouin oscillation in transparent free-standing diamond thin films in picosecond ultrasound
Source: arXiv:2203.05264 source file (2022-03-10)
Supplement: Supplementary file 1 [file Applied_Physics_Letters_Supplementary_Material.pdf]

SUPPLEMENTARY MATERIAL

# Suppression of Brillouin oscillation in transparent free-standing diamond thin films in picosecond ultrasound

H. K. Weng,[1] A. Nagakubo,[1] H. Watanabe,[2] and H. Ogi[1, a)]

[1)] *Graduate School of Engineering, Osaka University, 2-1 Yamadaoka, Suita, Osaka 565-0871, Japan*

[2)] *National Institute of Advanced Industrial Science and Technology, Tsukuba, Ibaraki 305-8568, Japan*

[a)] ogi@prec.eng.osaka-u.ac.jp

## Supplementary Figures

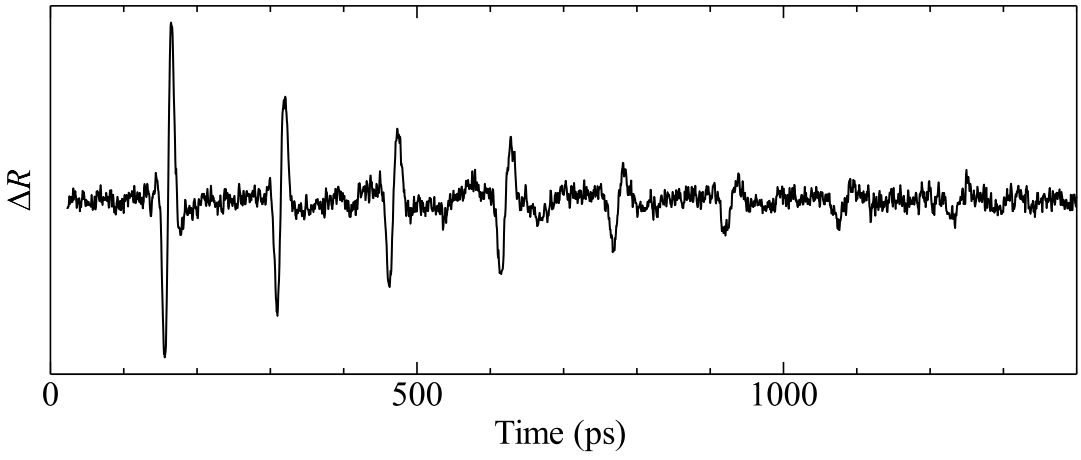


FIG. S1. The probe-light reflectivity change for a 350 nm thick graphite thin film. The background was subtracted.

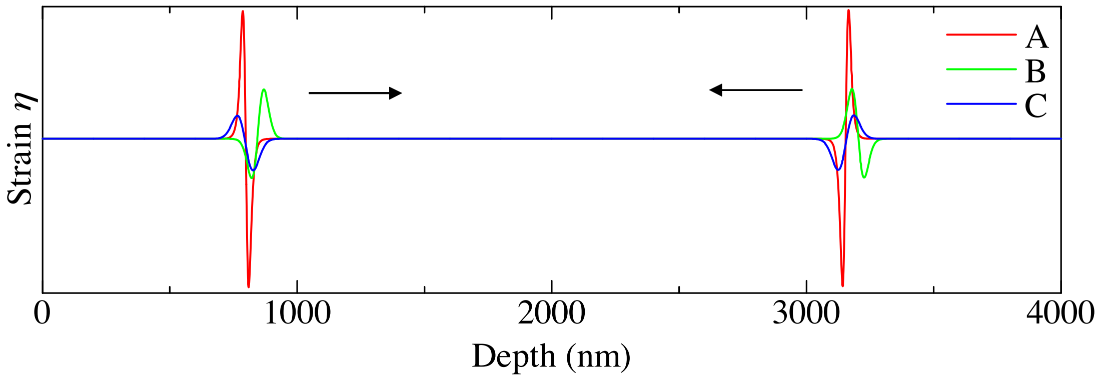


FIG. S2. The waveforms of the two strain pulses with $\Delta t$=2.74 ps. A, B, and C show the three time points in Fig. 2(b). The time instants are 45.7, 274.3, and 502.9 ps, respectively. (1/5, 6/5, and 11/5 of the single trip time, respectively) The arrows indicate the propagation direction of the strain pulses. Supplementary Movie 2 shows the details.

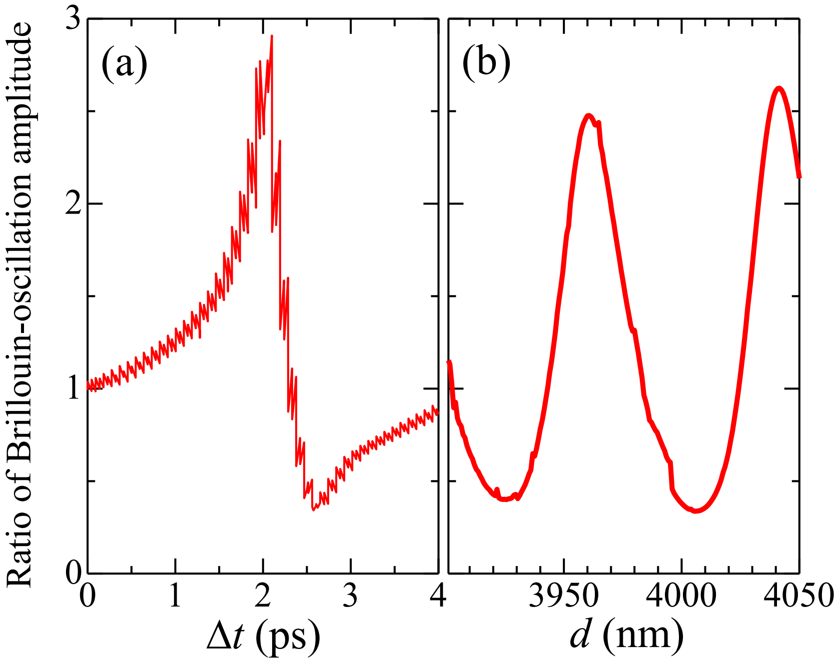


FIG. S3. Numerical simulations for dependence of the ratio of the Brillouin-oscillation amplitude after the first pulse echo to that before the first pulse echo on (a) the time delay for d=4000 nm and (b) the diamond-film thickness at $\Delta t$ = 2.74 ps. All parameters are the same as those used in Fig. 2, except for $\beta$ = 0.

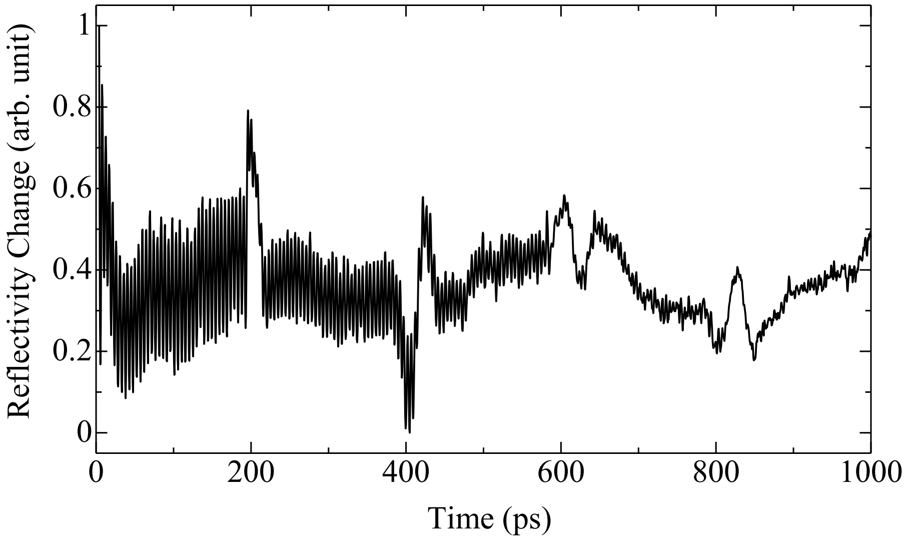


FIG. S4. An example of the observation in which the Brillouin oscillation does not disappear even when the Pt thin film is deposited on both sides (3.4 μm diamond free-standing film).
